# Supplementary material for: EigenPlaces: Training Viewpoint Robust Models for Visual Place Recognition
Source: arXiv:2308.10832 source file (2023-08-21)
Supplement: Supplementary file 1 [file supp_preds_grid.tex]

\begin{figure}
    \begin{center}
    \includegraphics[width=0.48\textwidth]{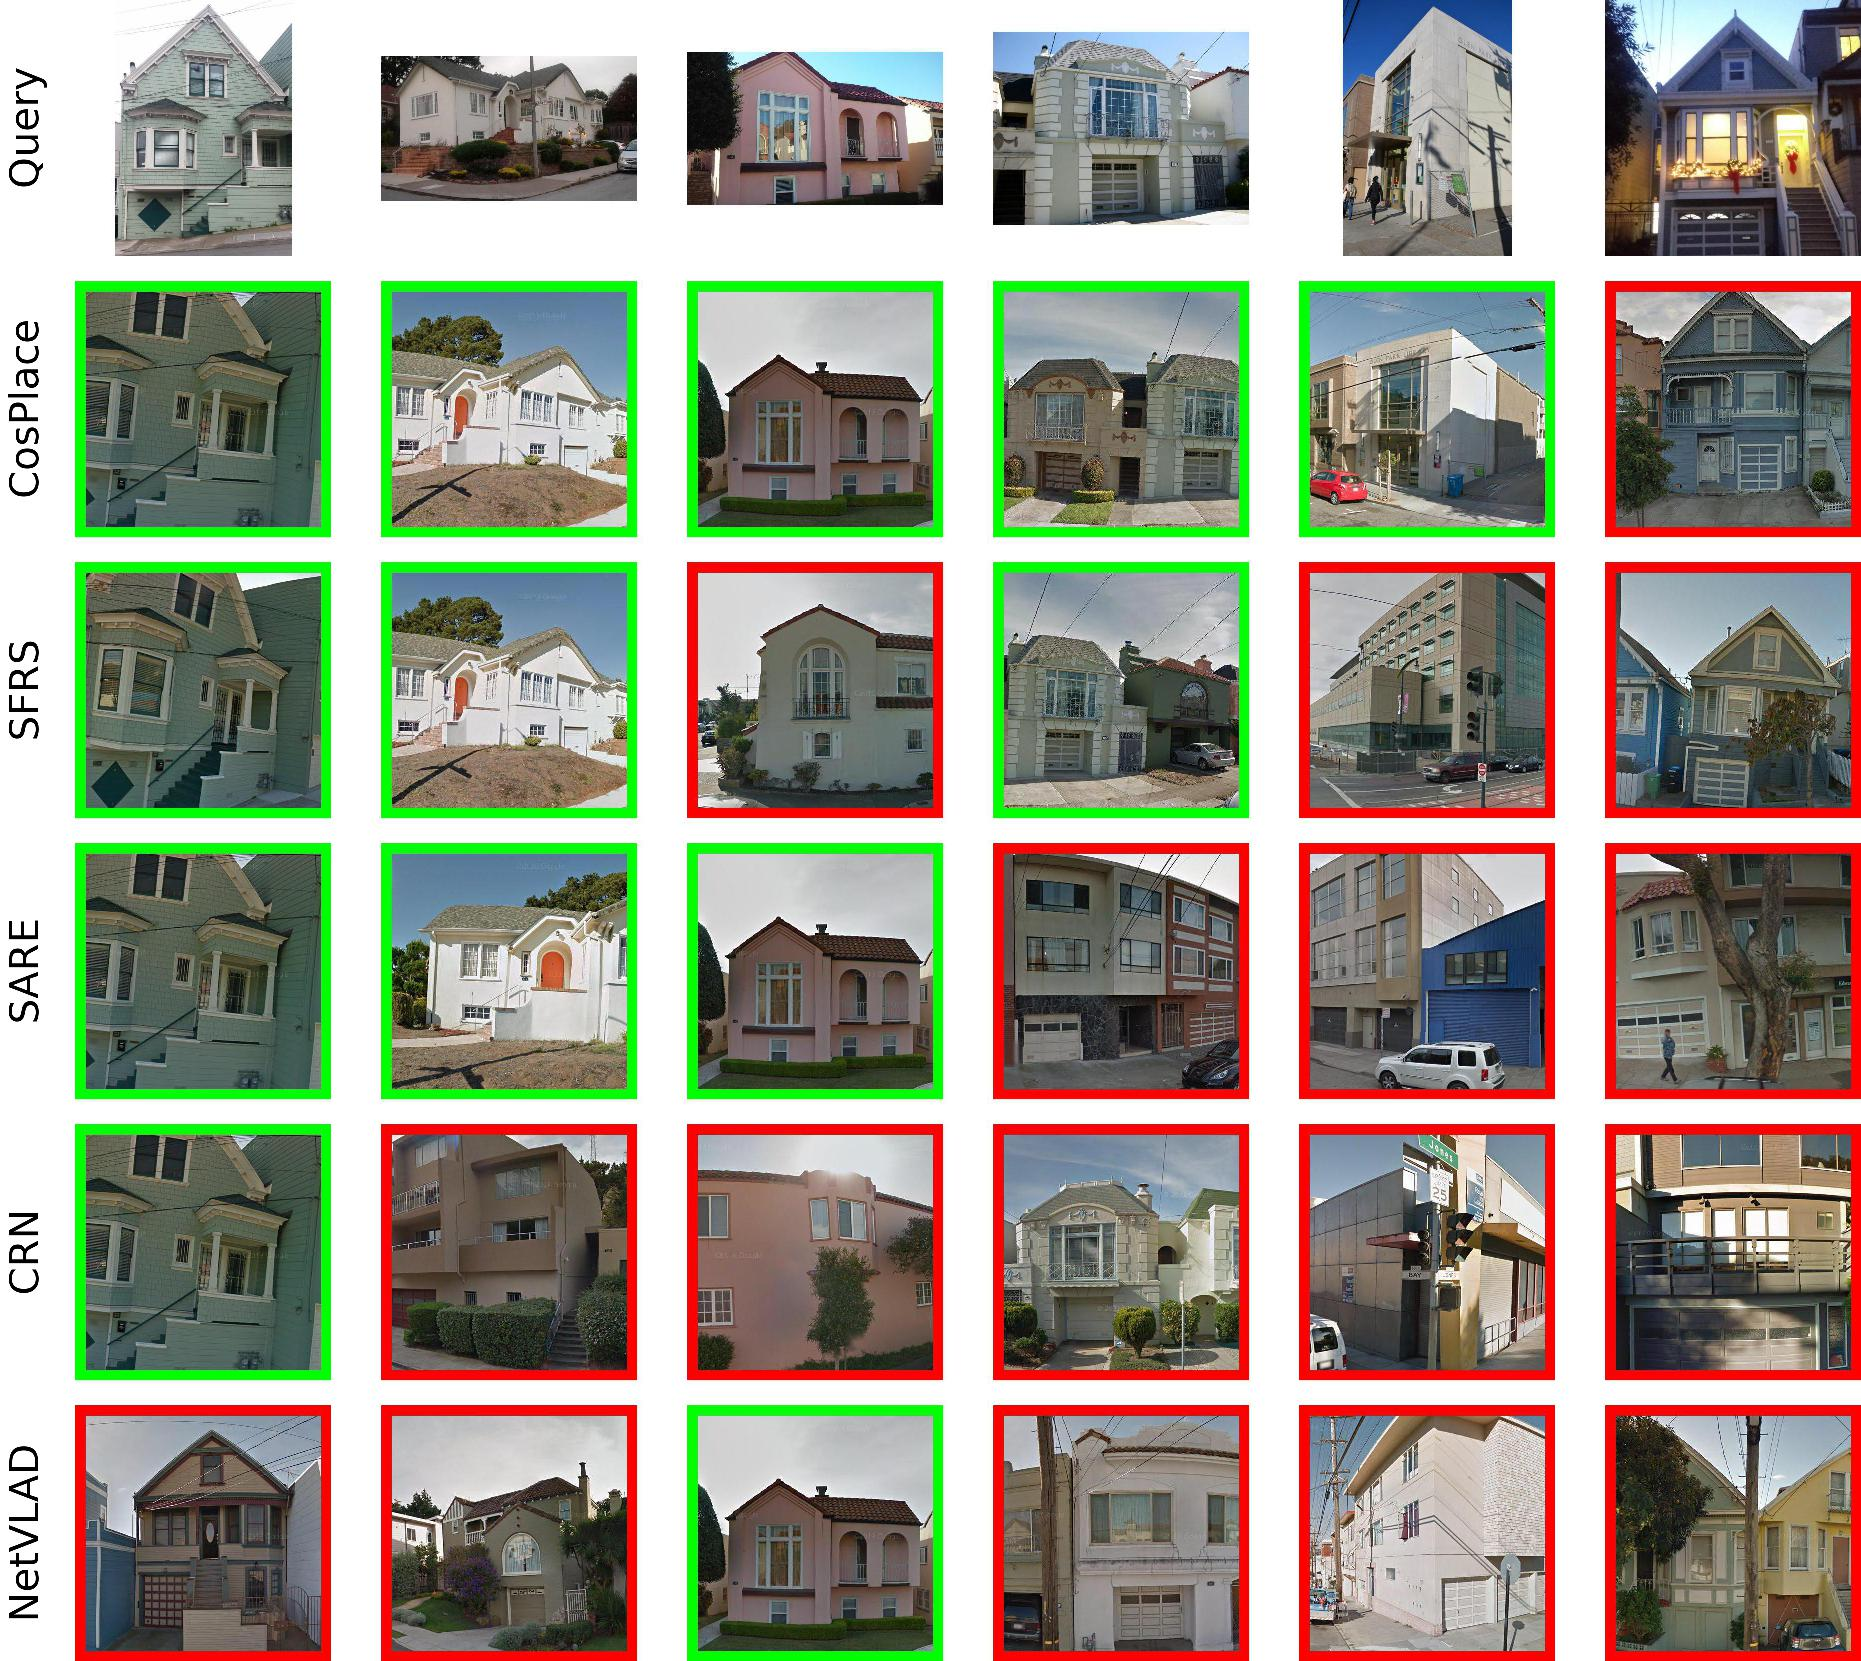}
    \end{center}
    \caption{
    \textbf{PLACEHOLDER COPIED FROM COSPLACE - TODO - Qualitative comparisons of retrieved images for a number of methods.}
    }
    \label{fig:preds_grid}
\end{figure}
